# Supplementary material for: Quantum magnetic imaging of current density in lithium-ion batteries
Source: arXiv:2512.01125 ancillary file (2025-11-30)
Supplement: Supplementary file 1 [file Supplementary_Information.pdf]

# Supplementary Information: Quantum magnetic imaging of current relaxation in lithium-ion batteries

W. Evans*,[1] T. Coussens,[2] M.T.M. Woodley,[2,3] A. M. Fabricant,[1] G. D. Kendall,[4]
M. Sonnet,[5,6] D. Wasylowski,[5,6] D. U. Sauer,[5,6,7] F. Oručević,[2] and P. Krüger[1,2,4]

[1] *Department of Biosignals, Physikalisch-Technische Bundesanstalt, 10587 Berlin, Germany*
[2] *Department of Physics and Astronomy, University of Sussex, Brighton, BN1 9RH, United Kingdom*
[3] *Centre for Photonics, Department of Physics, University of Bath, BA2 7AY, United Kingdom*
[4] *CDO2 Germany, Salzdahlumer Straße 196, 38126 Braunschweig, Germany*
[5] *Chair for Electrochemical Energy Conversion and Storage Systems (ESS) - Institute for Power Electronics and Electrical Drives (ISEA), RWTH Aachen University, Campus-Boulevard 89, 52074 Aachen, Germany*
[6] *Center for Ageing, Reliability and Lifetime Prediction of Electrochemical and Power Electronic Systems (CARL), RWTH Aachen University, Campus-Boulevard 89, 52074 Aachen, Germany*
[7] *Helmholtz Institute Münster: Ionics in Energy Storage (HI MS), IMD-4, Forschungszentrum Jülich, 52425 Jülich, Germany*

## Supplementary Note 1 - OPM setups and magnetic shielding

As discussed in the main text, modular OPM sensors were arranged in three different arrays/setups depending on the specific study:

- $4 \times 1$ array inside a table-top cylindrical shield, constructed from three layers of mu-metal, with inner diameter 0.5 m and length 1.0 m
- $2 \times 3$ array in the same table-top shield
- $4 \times 4$ array in the Berlin Magnetically Shielded Room (BMSR-2.1)

The BMSR-2.1 features a $3 \times 3 \times 3\,\mathrm{m}^3$ working space and is constructed from eight layers of mu-metal, in addition to a high-frequency aluminium shield. In Fig. S1, CAD renders of all OPM arrays and their respective 3D-printed holders are shown, with key characteristics summarized in Table S1.

The holders for the $4 \times 1$ and $2 \times 3$ OPM arrays were 3D-printed via fused deposition modeling (FDM) from high-temperature PLA material using an Ultimaker 3+ Extended. By contrast, measurements conducted with the $4 \times 4$ array in the BMSR-2.1 employed a larger frame with a reconfigurable array of sensors. The main rail system was constructed from FDM parts with ABS and PLA filament 3D-printed by a 3ntr A2v4, while the individual sensor holders were 3D-printed using a Formlabs Form3L using stereolithography (SLA) to print polypropylene-like Tough 1500 resin. This frame can hold up to 25 sensors and can be reconfigured to maximise coverage over different sample cells. The $4 \times 4$ OPM array allowed for eight sensors in two columns of four to measure the field directly above the cell, plus a column of four sensors on either side of the measurement field of view.

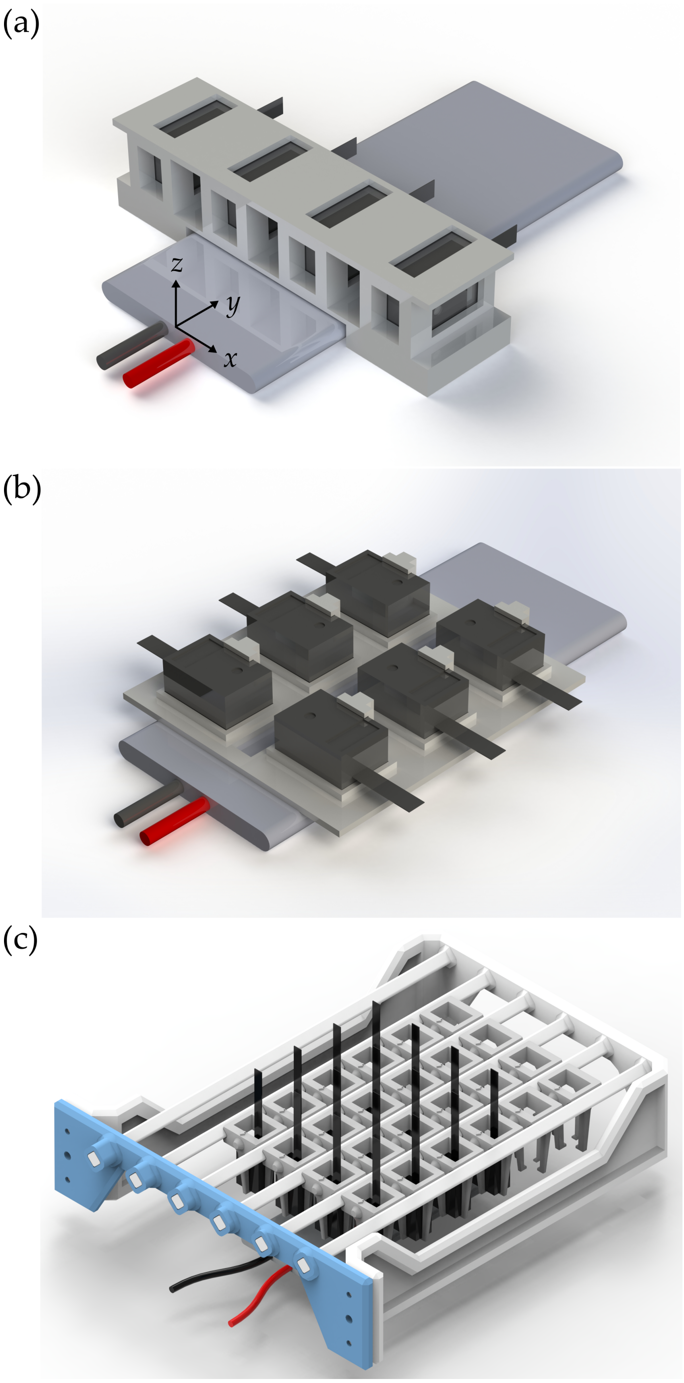


Figure S1 : CAD renders of (a) the $4 \times 1$ OPM array and holder, (b) the $2 \times 3$ OPM array and holder, and (c) the $4 \times 4$ OPM array and holder, each used for spatially resolved magnetic measurements of the $138.5 \times 58 \times 6\,\mathrm{mm}^3$ lithium polymer test cell. Main array parameters and sensitive measurement axes are listed in Table S1.

| **OPM array** | **Measured field components** | **Standoff distance (mm)** | **Inter-sensor spacing $x$,$y$ (mm)** |
|---|---|---|---|
| $4 \times 1$ [Fig. S1(a)] | $x$ and $y$ | 10.4 | 30, – |
| $2 \times 3$ [Fig. S1(b)] | $x$ and $z$ | 8.2 | 27, 30 |
| $4 \times 4$ [Fig. 1(a), Fig. S1(c)] | $y$ and $z$ | 8.4 | 30, 30 |

Table S1 : Overview of the three different OPM array configurations depicted in Fig. S1. For each case, the directions of magnetic-field sensitivity are listed according to the coordinate system in Fig. S1(a). Also indicated are the vertical stand-off distance from the battery surface to the centre of the sensing atomic vapour cell, and the spacing between sensors in the $x$-$y$ plane.

## Supplementary Note 2 - Computer tomography scanning

Two non-magnetic Powerstream flattened jelly-roll cells (PGEB-NM5858138-PCB) were used in this study. In order to better understand their internal structure, computer-tomography (CT) scans were conducted. Two cross-sections close to the cell terminals are shown in Fig. S2, where panels (a) and (b) focus on the current-collector tabs for the cathode and anode, respectively. The jelly-roll structure of the cell is clearly visible, where the repetition thickness (from one anode current collector to the next anode current collector) is approximately 340 µm.

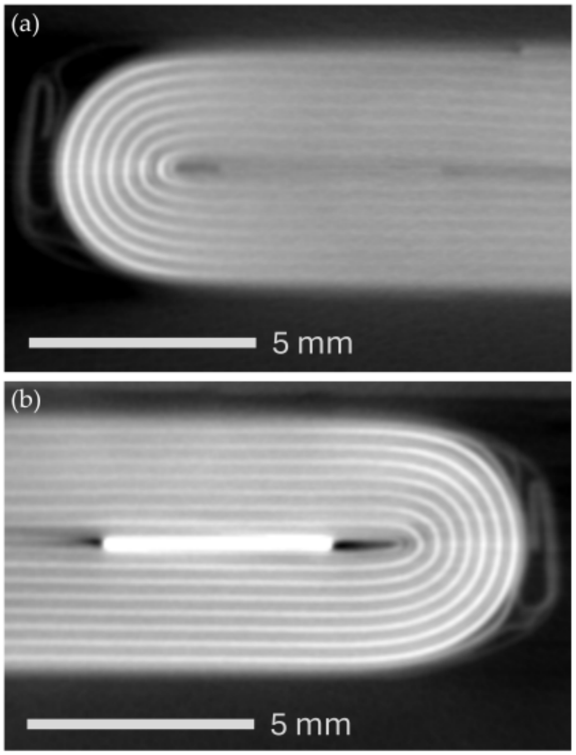


Figure S2 : CT scans showing cross-sections of the measured jelly-roll cell, close to the cell terminals. (a) focuses on the cathode's current-collector tab, while (b) focuses on the anode's current-collector tab.

## Supplementary Note 3 - Finite-Element Simulations

A full three-dimensional simulation of the jelly-roll cell, including current density and the associated magnetic field, would be extremely complex and computationally expensive. In order to reduce the calculation time, a single layer was simulated and this simulation was split in two. The current density was computed in the COMSOL finite-element simulation software, Version 6.1, using the 'Electrode Utilization in a Large-Format Lithium-Ion Battery Pouch Cell' template model from the Battery Design Module. The magnetic field was then calculated in MATLAB from the exported current-density COMSOL simulation. A summary of parameters used in the three-dimensional current-density simulation is presented in Table S2.

To reduce simulation time while analysing the dependence on discharge time, current, and state of charge (Fig. S3), a one-dimensional model was employed to simulate the electrochemical behaviour of the cell along the electrode thickness. This was also computed in COMSOL using a modified version of the 'Lithium-Ion Battery Internal Resistance' template model from the Battery Design Module, which calculates the mass and charge transport in the liquid electrolyte within the porous structure of the active material, including the intercalation reactions and internal particle diffusion. A summary of parameters used in the one-dimensional simulation is presented in Table S3.

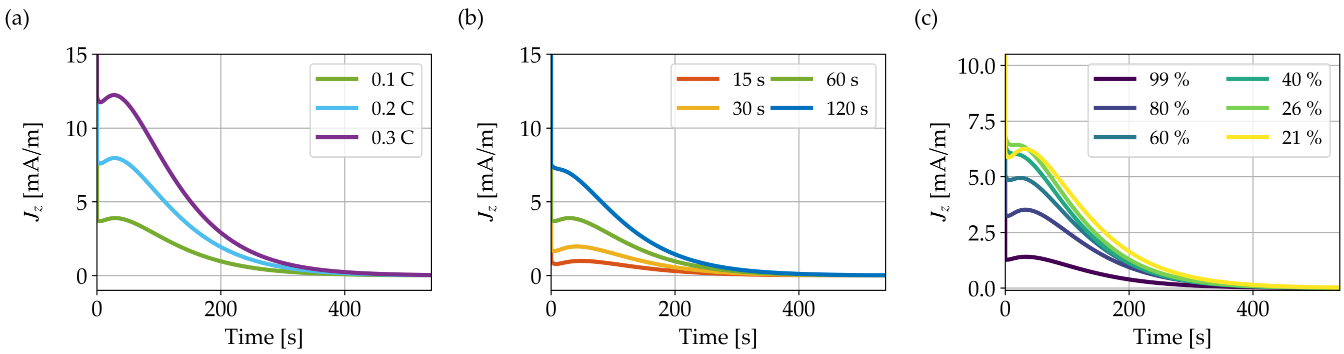


Figure S3 : (a) Simulated electrolyte current density in the positive electrode 20 µm from the electrode-separator boundary, according to a one-dimensional finite-element simulation. The plotted curves correspond to 60 s discharge pulses of increasing current: 0.6 A (0.1 C), 1.2 A (0.2 C), and 1.8 A (0.3 C). (b) Results of the same simulation as in (a) but for increasing discharge times of a 0.6 A (0.1 C) pulse: 15 s, 30 s, 60 s, and 120 s. (c) Simulated electrolyte current density shown for SoC between 21% and 99%. Unlike in the experimental data (Fig. 5 in the main text), the qualitative shape of the simulated current density stays consistent across different SoC, even though there is a significant drop in peak amplitude of the current density between 99% and 21% SOC.

| **Name** | **Value** | **Description** |
|---|---|---|
| $M_{\text{Neg}}$ | Graphite Electrode, LixC6 MCMB (Negative, Li-ion Battery) | Negative electrode material |
| $M_{\text{Pos}}$ | NMC Electrode, LiNi1/3Mn1/3Co1/3O2 (Positive, Li-ion Battery) | Positive electrode material |
| $M_{\text{E}}$ | LiPF6 in 1:2 EC:DMC and p(VdF-HFP) (Polymer electrolyte, Li-ion Battery) | Electrolyte material |
| $M_{\text{PCC}}$ | Aluminium | Positive current collector material |
| $M_{\text{NCC}}$ | Copper | Negative current collector material |
| $L_{\text{sep}}$ | $30 \times 10^{-6}$ m | Separator thickness |
| $L_{\text{pos}}$ | $60 \times 10^{-6}$ m | Positive electrode thickness |
| $L_{\text{neg}}$ | $60 \times 10^{-6}$ m | Negative electrode thickness |
| $L_{\text{poscc}}$ | $10 \times 10^{-6}$ m | Positive current collector thickness |
| $L_{\text{negcc}}$ | $10 \times 10^{-6}$ m | Negative current collector thickness |
| $W_{\text{cell}}$ | 0.06 m | Cell width |
| $H_{\text{cell}}$ | 0.138 m | Cell height |
| $H_{\text{tab}}$ | 0.007 m | Tab height |
| $W_{\text{tab}}$ | 0.1 m | Tab width |
| $r_{\text{p\_pos}}$ | $2 \times 10^{-6}$ m | Positive electrode particle radius |
| $r_{\text{pneg}}$ | $5 \times 10^{-6}$ m | Negative electrode particle radius |
| $\text{cs}_{\text{maxpos}}$ | 22860 mol/m$^3$ | Maximum host capacity, positive electrode |
| $\epsilon_{\text{spos}}$ | 0.5 | Positive electrode porosity |
| $Q_{\text{cell}}$ | 224.63 C | Capacity of simulated cell geometry |
| $cs_{\text{maxneg}}$ | 31507 mol/m$^3$ | Maximum host capacity, negative electrode |
| $\epsilon_{\text{sneg}}$ | 0.45347 | Negative electrode porosity |
| $I_{1C}$ | 0.062398 A | Cell 1C current for this geometry |
| $\text{SoC}_{\text{maxpos}}$ | 0.995 | Local SOC in positive electrode at 0% cell SoC |
| $\text{SoC}_{\text{maxmin}}$ | 0.175 | Local SOC in positive electrode at 100% cell SoC |

Table S2 : Parameters used in the 3D finite-element simulation of a single-layer cell.

| **Name** | **Value** | **Description** |
|---|---|---|
| $M_{\text{Neg}}$ | Graphite Electrode, LixC6 MCMB (Negative, Li-ion Battery) | Negative electrode material |
| $M_{\text{Pos}}$ | NMC Electrode, LiNi1/3Mn1/3Co1/3O2 (Positive, Li-ion Battery) | Positive electrode material |
| $M_{\text{E}}$ | LiPF6 in 1:2 EC:DMC and p(VdF-HFP) (Polymer electrolyte, Li-ion Battery) | Electrolyte material |
| $L_{\text{sep}}$ | $30 \times 10^{-6}$ m | Separator thickness |
| $L_{\text{pos}}$ | $60 \times 10^{-6}$ m | Positive electrode thickness |
| $L_{\text{neg}}$ | $60 \times 10^{-6}$ m | Negative electrode thickness |
| $Q_{\text{Cell}}$ | 224.63 C | Battery capacity |
| $\text{rp}_{\text{pos}}$ | $2 \times 10^{-6}$ m | Particle size positive electrode |
| $\text{epsl}_{\text{pos}}$ | 0.5 | Porosity positive electrode |

Table S3 : Parameters used in the 1D finite-element simulation of a single-layer cell.

For the magnetic-field simulations (Figs. S4–S5), the Biot-Savart law was used:

$$\mathbf{B}(\mathbf{r}) = \frac{\mu_0}{4\pi} \int_V \frac{\mathbf{J}(\mathbf{r}') \times (\mathbf{r} - \mathbf{r}')}{|(\mathbf{r} - \mathbf{r}')|^3} \, d^3\mathbf{r}', \tag{1}$$

where $\boldsymbol{B}(\boldsymbol{r})$ is the magnetic flux density at position $\boldsymbol{r}$, due to current density distribution $\mathbf{J}(\mathbf{r}')$ at position $\boldsymbol{r'}$, with $\mu_0$ being the vacuum magnetic permeability.

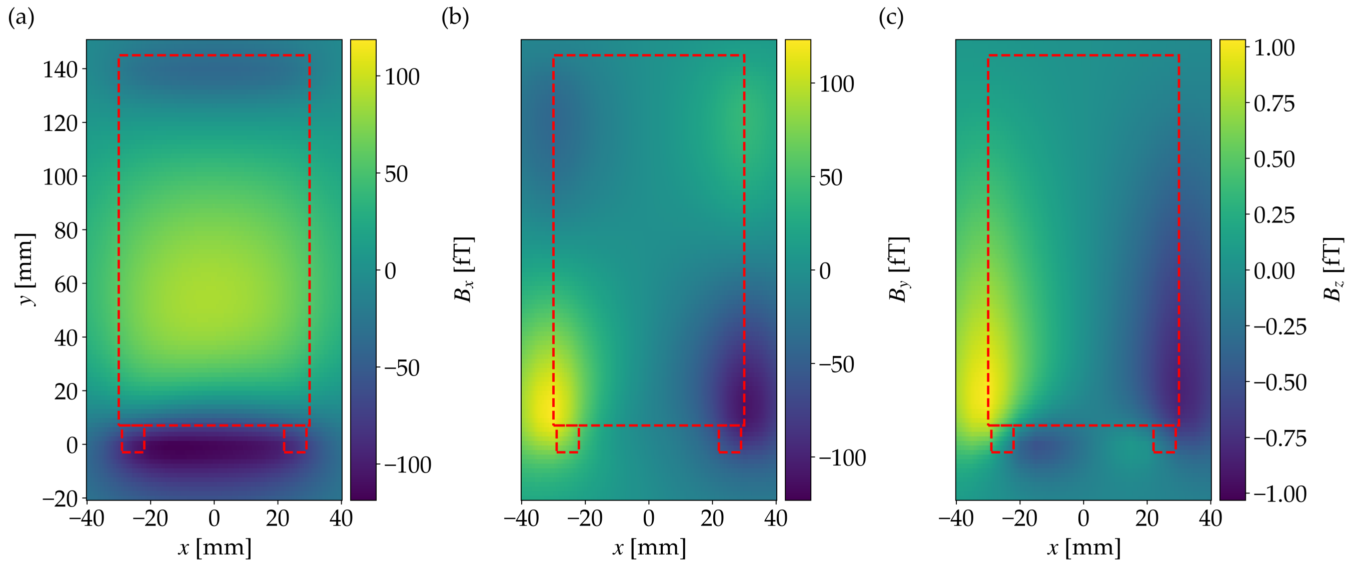


Figure S4 : Simulated images showing the (a) $x$-component, (b) $y$-component and (c) $z$-component of the magnetic field produced by current in the electrolyte, as obtained from finite-element simulations of the cell with 62.4 mA h-capacity after pulsed discharge. Red dashed lines indicate the spatial position and extent of cell. Images are taken 0.5 s after the end of the pulse during the first peak in current density, revealing spatial variation of transient relaxation activity—panel (a) shows that the $x$-component of the magnetic field has a strong gradient along the length of the cell, whereas panels (b) and (c) show large gradients at the side edges of the cell.

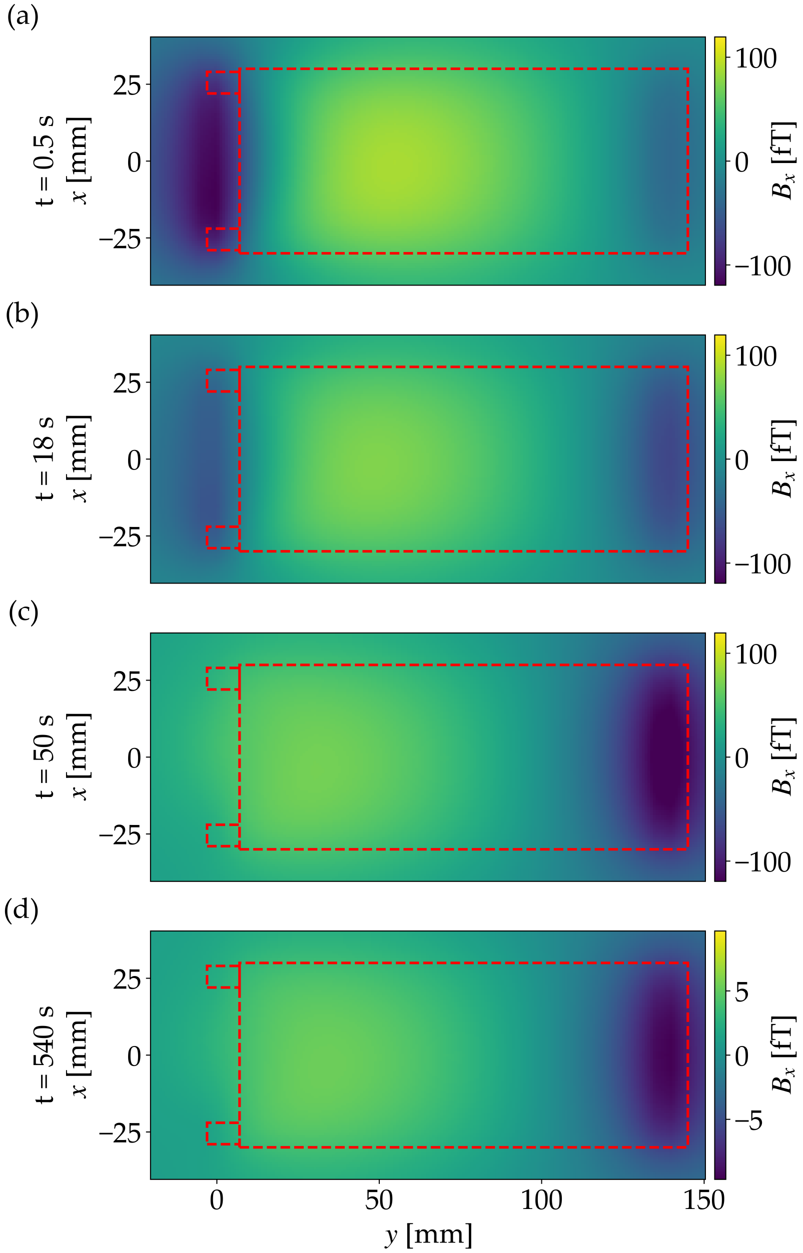


Figure S5 : Images showing time evolution of the $x$-component of the magnetic field produced by current in the electrolyte, as obtained from finite-element simulations of a cell with 62.4 mA h-capacity after pulsed discharge. Here we see the $B_x$ field, resultant from currents in the $y$- and $z$-directions, 8 mm above the cell at times between 0.5 s and 540 s after the discharge pulse. The topmost panel (same as the leftmost panel of Fig. S4) shows a snapshot at 0.5 s after switching off the current and predicts a strong gradient along the length of the cell. The lower panels capture the current density at 18 s, 50 s, and 540 s after the end of the pulse, capturing the peak in current density. Note that the colour scaling of the image in the bottom panel is reduced for visualisation, due to overall decay of the current distribution at longer timescales.

## Supplementary Note 4 - Relaxation Data Fitting Procedure

For all six sensors in the $2 \times 3$ array (Fig. S1(b)), the amplitudes $A_i$ and the relaxation times $\tau_i$ are extracted using the fit function

$$B(t) = A_1 e^{-t/\tau_1} + A_2 e^{-t/\tau_2} + A_3 e^{-t/\tau_3} + mt + c\,. \tag{2}$$

Before the exponential fitting is undertaken, a linear fit is performed to subtract offsets ($c$) and drifts ($mt$) using data from the end of the dataset (599 s to 899 s). As sums of exponentials may otherwise yield non-unique solutions, the fitting procedure leverages the distinct timescales (fast on order 1 s, intermediate on order 10 s, and slow on order 100 s) of each exponential and determines their parameters sequentially to ensure a unique solution. The slowest-timescale exponential, defined as $A_3 e^{-t/\tau_3}$, is first fitted to the data omitting the initial 100 s, with bounds set to be $-700 < A_3 < 700$ and $80 < \tau_3 < 200$. After determining its parameters, this component is fixed and its contribution is removed from the signal. The intermediate-timescale exponential ($A_2 e^{-t/\tau_2}$) is then fitted excluding the first 15 s of data, with bounds set to be $-700 < A_2 < 700$ and $\tau_2 < 40$. Finally, with both the long- and medium-timescale parameters fixed and contributions removed, the fast-timescale exponential ($A_1 e^{-t/\tau_1}$) is fitted using the full dataset with bounds set to be $-700 < A_1 < 700$ and $\tau_1 < 12$. Parameter sets are excluded whenever any individual parameter reaches its prescribed bounds.

Not all three exponential components appear at every position or state of charge. To avoid over-fitting, each shorter-timescale component ($A_2 e^{-t/\tau_2}$ and $A_1 e^{-t/\tau_1}$) is added sequentially to the total fit, but is omitted whenever its inclusion increases the $R^2$ of the fit by less than $5 \times 10^{-5}$. Where repeat measurements and fitting procedures were performed at the same SoC, each data point represents the mean of the extracted parameters, and the error bars reflect the minimum to maximum variation. Data points which exhibit no error bars are derived from a single dataset.
